# Supplementary material for: SEW: Self-calibration Enhanced Whole Slide Pathology Image Analysis
Source: arXiv:2412.10853 source file (2025-02-14)
Supplement: Supplementary file 1 [file X_suppl.tex]

\clearpage
\setcounter{page}{1}
\maketitlesupplementary

In this supplementary material, we provide detailed information on the pathological datasets used for diagnosis and prognosis (\emph{Section} A), the SEW training pipeline(\emph{Section} B), additional focus heatmaps and visualizations of the clustering results from the local branch(\emph{Section} C). The source code is also provided in the ``\emph{code.zip}'' file.

\begin{algorithm*}[!t]
  \caption{The training pipeline of Self-calibration Enhanced Whole Slide Pathology Image Classification.}
  \label{alg:sew}
  \LinesNumbered
  \KwIn{A dataset of pathological slide images $\{\mathcal{I}, y_{gt}\}$, the GCN network $ f_{\text{GCN}}^{\text{global}} $ and the transformer encoder $f^{\text{global}}_{\text{Atten}}$ for the global branch, the focus predictor $f_{\text{MLP}}^{\text{focus}}$, the GCN network $f_{\text{GCN}}^{\text{local}}$;}
  \KwOut{The trained modules of the SEW;}
  \BlankLine
  \textbf{Initialization:}$f_{\text{GCN}}^{\text{global}} , f^{\text{global}}_{\text{Atten}}$, $f_{\text{MLP}}^{\text{focus}}$, $f_{\text{GCN}}^{\text{local}};$\\
    % \While{\textnormal{local branch is not converged}}{
    \For{each slide $\mathcal{I}$}{
        Building superpixel graph $\mathcal{G}_{\text{global}}(\mathcal{V},\mathcal{E})$\\
        Calculating node embedding $ [ h_1, h_2, ..., h_N] $ with $f_{\text{GCN}}^{\text{global}}(\mathcal{G}_{\text{global}})$\\
        Calculating $\text{CLS}'_{\text{global}}$ with $ f^{\text{global}}_{\text{Atten}}([h_1,..., h_N, \text{CLS}_{\text{global}}]))$\\
        Global branch prediction $y'_{cls}=f^{\text{global}}_{\text{MLP}}(\text{CLS}'_{\text{global}})$\\
        Minimizing the global branch loss $ \mathcal{L}_{cls}^{global} = CE(y'_{cls},y_{gt})$\\
        \If{\textnormal{global branch is converged}}{
            Calculating focus score $q'_n$ on $f_{\text{MLP}}^{\text{focus}}([h'_1, h'_2, ...,h'_N]),     [h'_1, ..., h'_N, \text{CLS}'_{\text{global}}] =f^{\text{global}}_{\text{Atten}}([h_1,..., h_N, \text{CLS}_{\text{global}}])$\\
            selecting Top-K sub-graph
            $\{\mathcal{G}_{\text{sub}}^k(\mathcal{V}^k,\mathcal{E}^k)\}_{k=1}^K$\\
            \For{ each sub-graph $\mathcal{G}^k_{\text{sub}}$}{
                 %Amplified  $\mathcal{G}_{\text{sub}}$ as  $\mathcal{G}_{\text{local}}$\\
                 Obtaining $T$ node groups $\{\{u^t_j\}^J_{j=1}\}^T_{t=1}$  from sub-graph $\mathcal{G}^k_{\text{sub}}$\\
                Calculating node embedding $ [ r^t_1, r^t_2, ..., r^t_J] &= \text{Norm}(W^{\text{proj}}_{local}[u^t_1, u^t_2, ..., u^t_J]), 
    W^{\text{proj}}_{local} & \in \mathbb{R}^{J \times J}, u^t_j \in \mathbb{R}^{1 \times d} $ \\
                Calculating intra-group class token $\text{CLS}'^t_{\text{local}} = \text{GroupAtten}([ r^t_1, r^t_2, ..., r^t_J], \text{CLS}^t_{\text{local}})$\\
                Calculating inter-group class token $\overline{\text{CLS}}^t_{\text{local}} = \text{Atten}(\{\text{CLS}'^t_{\text{local}}\}^T_{t=1},\text{CLS}'^t_{\text{local}})$ \\
                Obtaining the local branch prediction $\overline{y}^t=f^{\text{local}}_{\text{MLP}}( \overline{\text{CLS}}^t_{\text{local}})$\\
                Minimizing the local branch prediction loss $ \mathcal{L}^{local}_{\text{CLS}} =\frac{1}{T} \sum_{t=1}^T \text{CE}(\overline{y}^t,y^t_{gt})$\\
                
                Minimizing the global and local consistency constraint loss $ \mathcal{L}^{\text{cst}} = D_{KL}(W^{\text{proj}}_{cls} \overline{\text{CLS}}^t_{\text{local}} || h'_n)$\\
                Minimizing the focus predictor loss $  \mathcal{L}^{focus} = D_{KL}(Q'_{focus}||Q_{gt}), Q'_{focus}=\{q'_n \}^N_{n=1}$\\
                Obtaining the pathological prototype vocabulary $\{O_{c}\}^C_{c=1}$
            }
            Obtaining the mixture feature $H_{all} &= W^{\text{mapping}}_{global} \text{CLS}_{global} +W^{\text{mapping}}_{local} \frac{1}{K} \sum^K_{k=1} \text{CLS}^k_{local} +W^{\text{mapping}}_{proto} \frac{1}{C} \sum^C_{c=1} O_{c}$\\
            Making the final prediction $y'_{final}= f^{\text{all}}_{\text{MLP}}(H_{all})$\\
            Minimizing the final loss $\mathcal{L}^{all}=CE(y'_{final},y_{gt})$

        }
    }
\end{algorithm*}
\section*{A. Dataset Details}
\label{datasetDetails}
The experiments in this paper are conducted on the following datasets, including diagnostic grading datasets (CAMELYON16~\cite{camelyondataset}, PANDA~\cite{pandadataset}, BRCA\cite{lingle2016cancer}, GC) and prognostic datasets (LUAD\cite{albertina2016cancer}, HCC, CRC). HCC, GC, and CRC are datasets collected in this work, with each slide coming from real cases and annotated by professional pathologists for lesion areas and categories. CAMELYON16, PANDA, BRCA, and LUAD are all public datasets.

The amount of slides in each dataset is counted as follows. CAMELYON16 is a breast cancer dataset with two-category labels, including $159$ negative slides and $111$ positive slides. The $PANDA$ dataset is a prostate cancer dataset, containing $10516$ slides. These grades are determined based on the Gleason system~\cite{EPSTEIN2010433}., which can reflect prognostic information. BRCA is a public breast cancer dataset from TCGA; we filtered out the inaccurately annotated data, and finally used 591 negative slides and $267$ positive slides. For prognosis prediction, the LUAD dataset includes the survival status of patients at follow-up. To be rigorous, negative samples followed up within 100 days after surgery were excluded. Finally, there are $227$ negative slides and $127$ positive slides. In addition, the HCC dataset contains $117$ slides of hepatocellular carcinoma, divided into 5 different levels according to the follow-up prognosis. The CRC dataset contains 343 slides of colorectal cancer, divided into two categories based on the follow-up prognosis. The GC dataset contains 343 slides of gastric cancer, divided into five categories according to the type of pathological diagnosis.Additional statistical information is presented in Figure~\ref{fig:dataset}.

\section*{B. Network Architecture}
\label{Architecture}
After extensive experiments, we found that a simple super-pixel graph classifier architecture is sufficient to meet the focusing and classification requirements on pathological datasets.
The SEW has two independent branches with separate parameters. The construction of the super-pixel graph uses the SLIC algorithm, and the process of extracting node embeddings uses a three-layer GCN network, with each node's feature dimension set to 384. For the global branch, the attention module is implemented with a transformer that includes a cls token, with a depth of 12. For the local branch, the intra-group attention module uses a transformer with a group token, with a depth of 8. The inter-group attention module uses a transformer without any tokens, also with a depth of 8. All transformers used in this paper have an embedding dimension of 384, equipped with 6 attention heads. The node representation output from the global branch's transformer is used as the input for the classifier and focusing predictor, which includes two fully connected layers with an intermediate dimension of 192. The GeLU activation function~\cite{hendrycks2016gelu} is used. Their output dimensions are the category number C and 1, respectively. The architectural details of SEW are found in the code of the supplementary materials. The workflow of SEW is shown in the Algorithm~\ref{alg:sew}.

\begin{figure*}[!h]
    \includegraphics[width=0.95\textwidth]{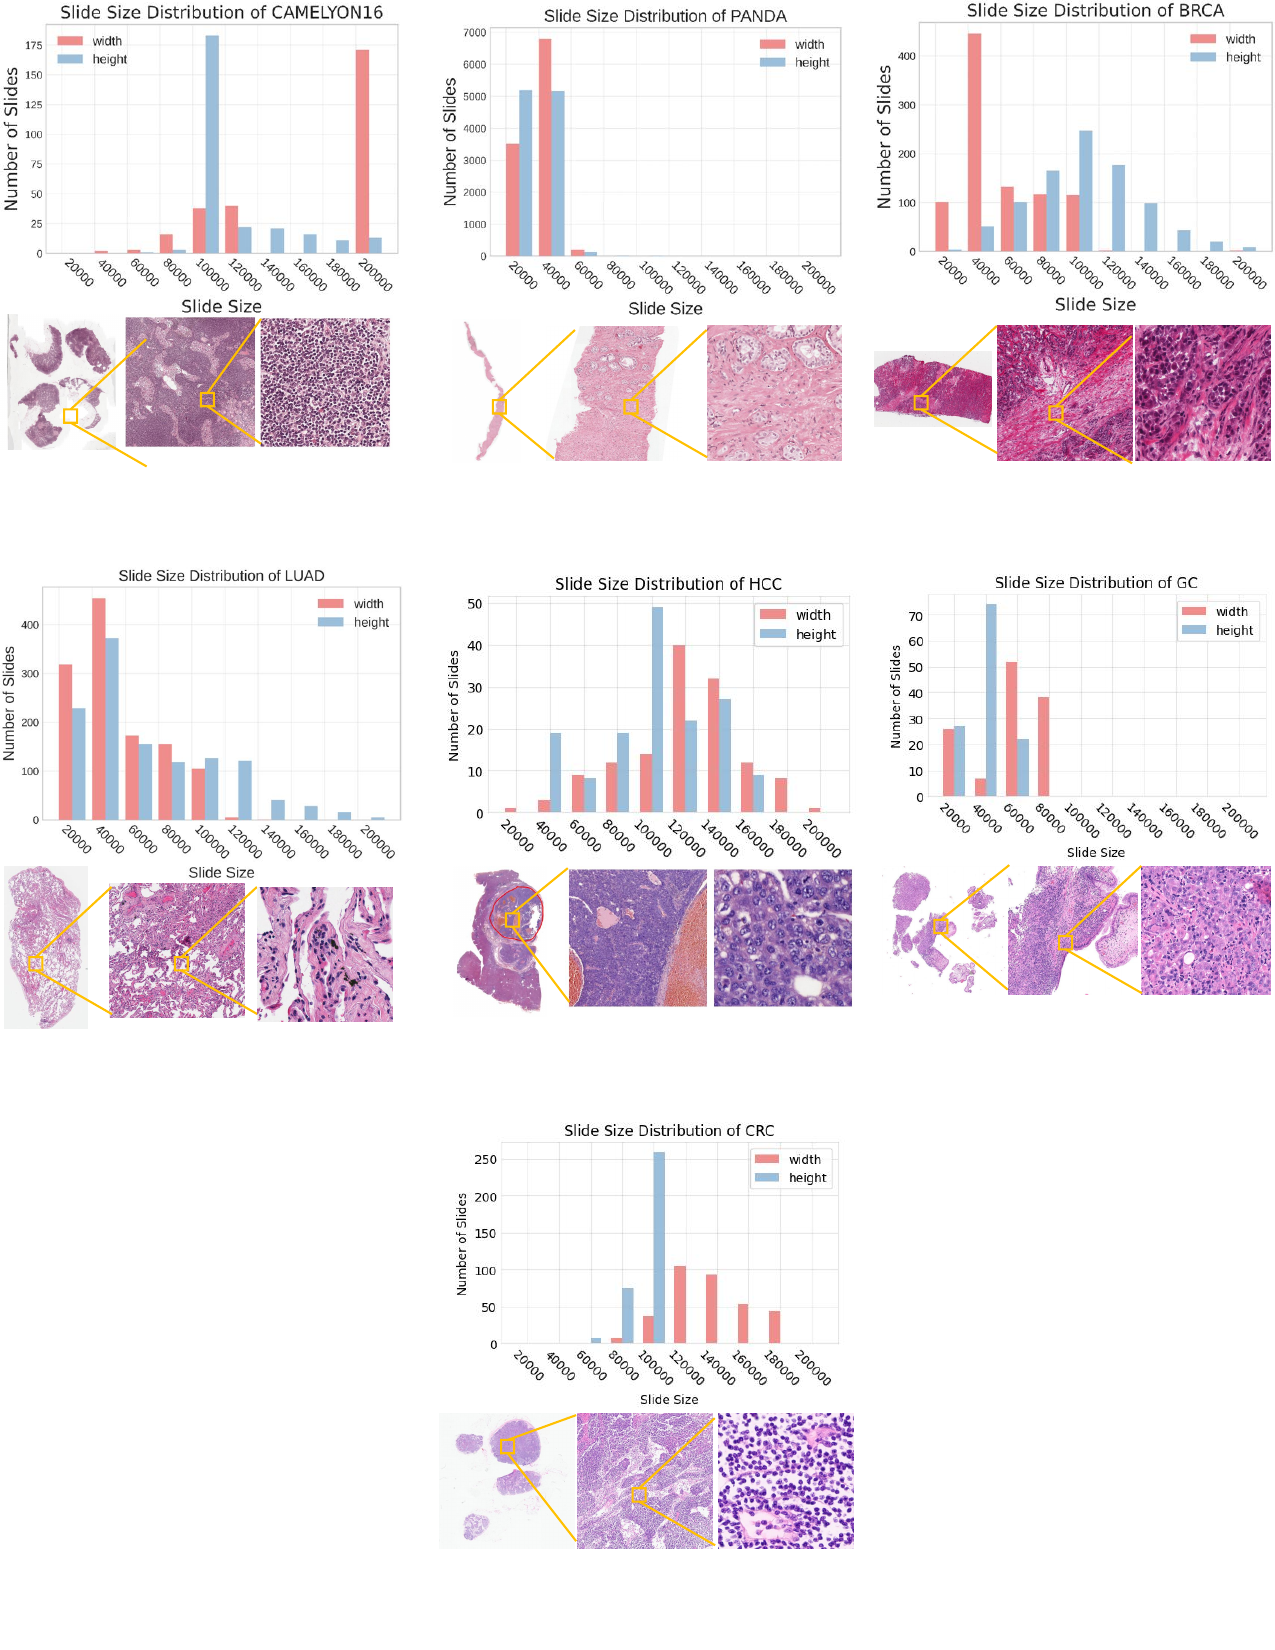}
    \caption{The size statistics of the seven datasets used in this paper, as well as schematic diagrams at different magnifications.} 
    \label{fig:dataset}
\end{figure*}
\begin{figure*}[!h]
    \includegraphics[width=0.92\textwidth]{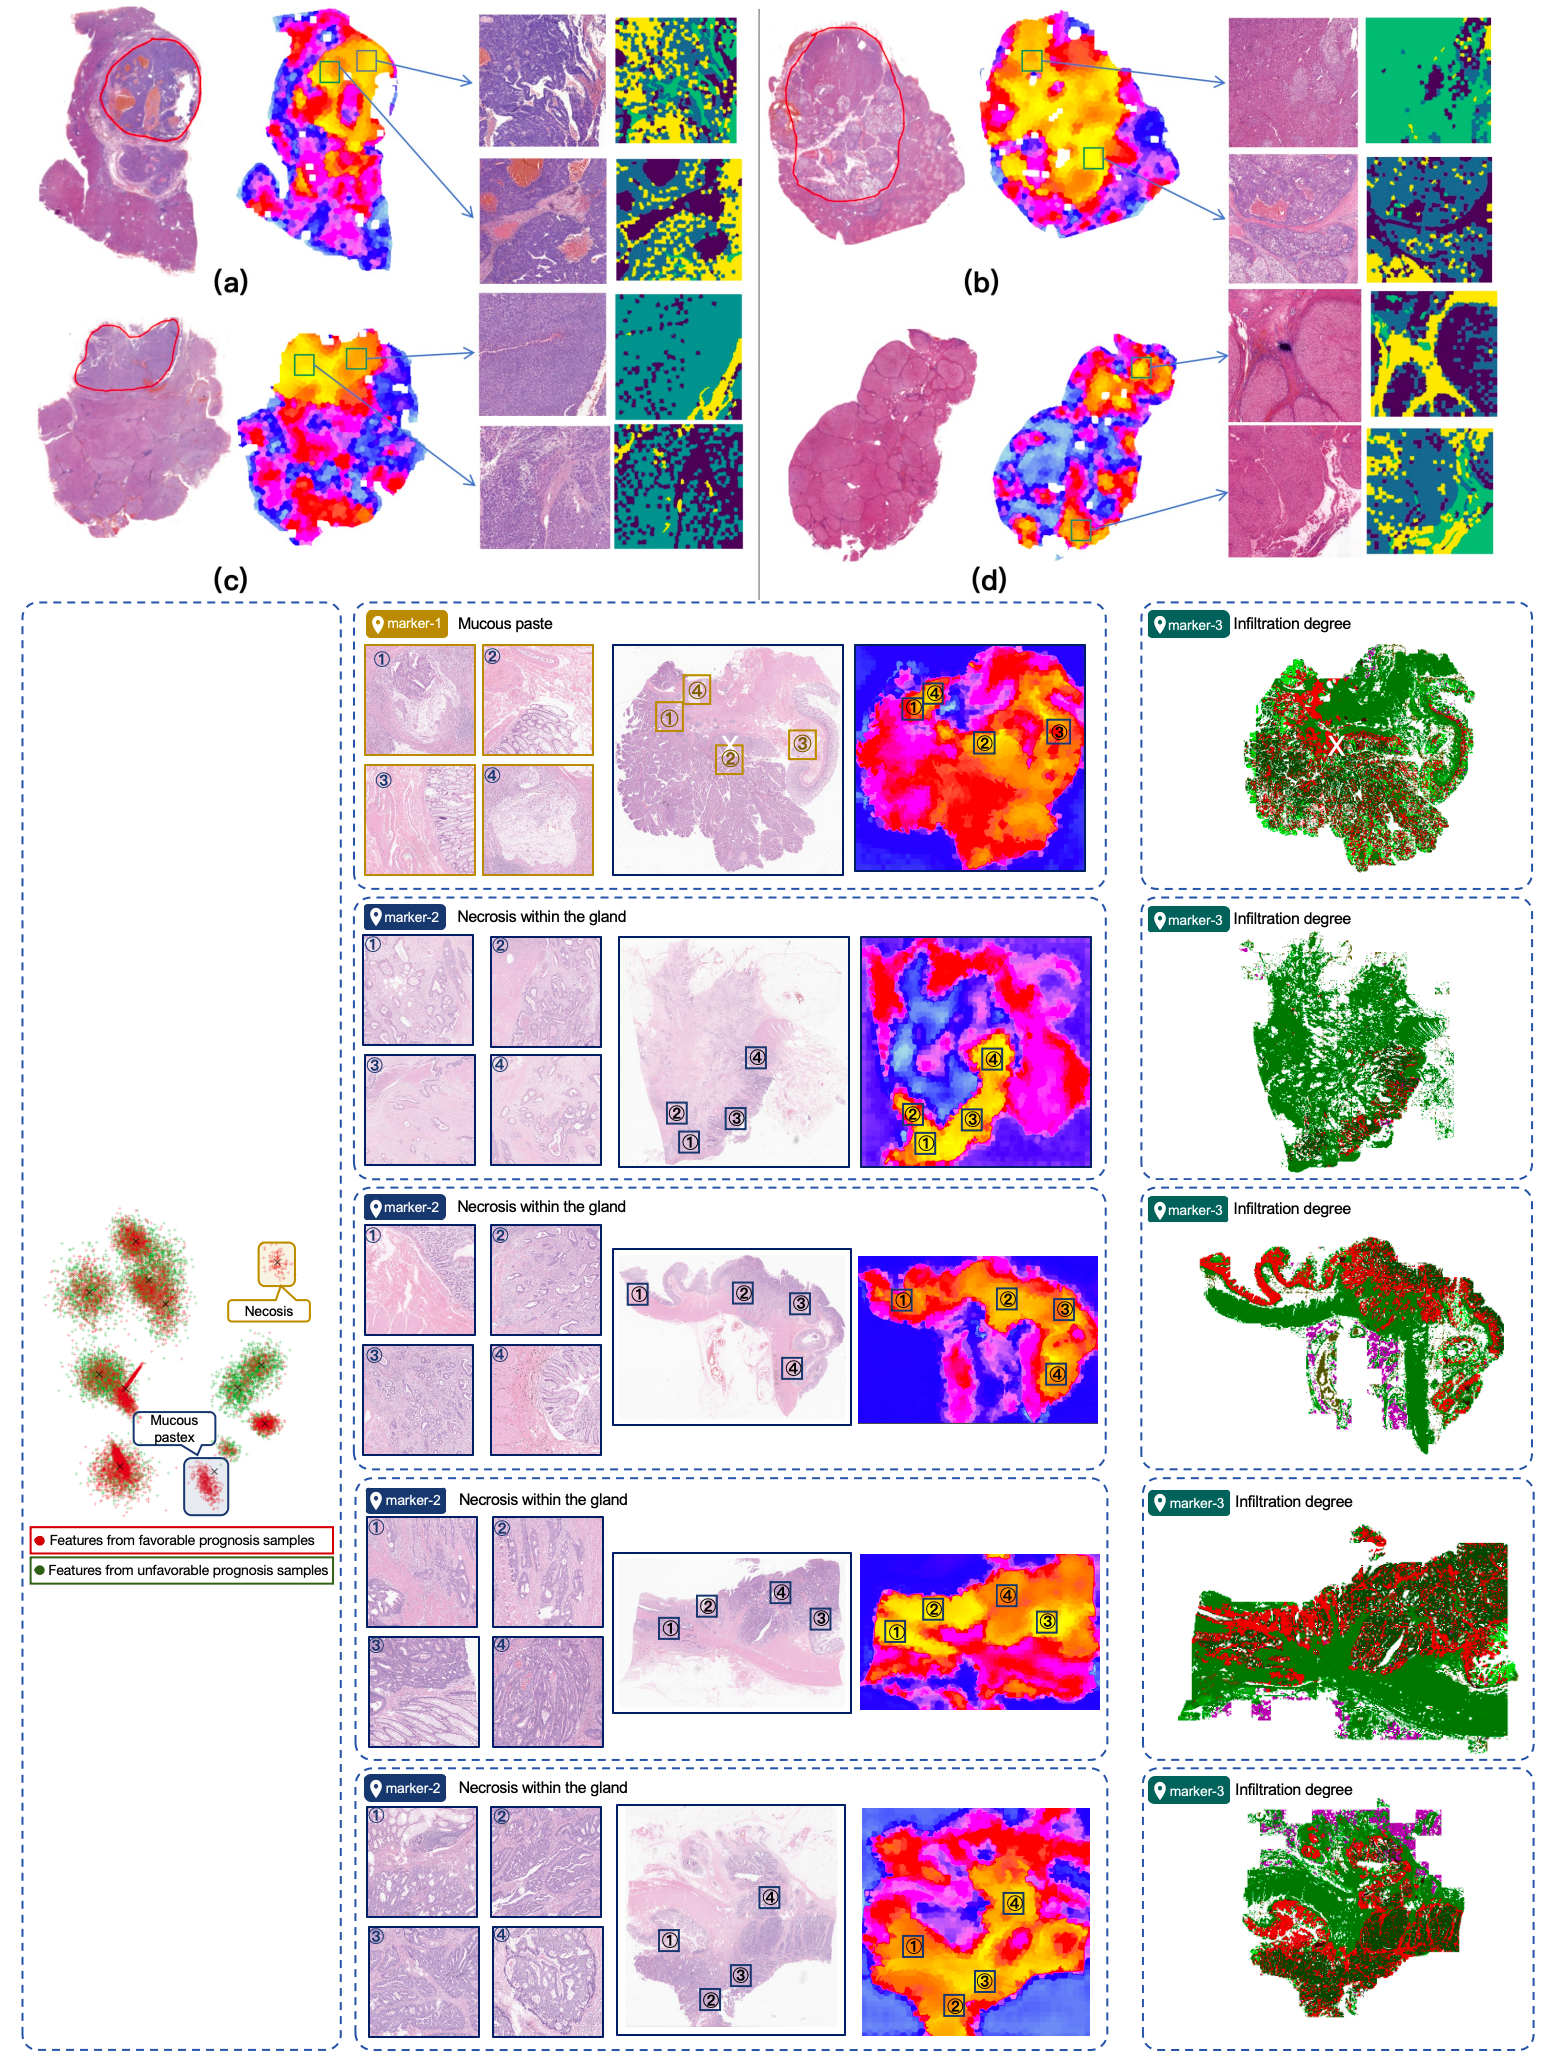}
    \caption{
    The visualization of WSI, heatmap predicted by focus predictor, critical patches and the explainable tissue map constructed with pathological prototype vocabulary.
    } 
    \label{fig:visual2}
\end{figure*}
\begin{figure*}[!h]
    \includegraphics[width=0.98\textwidth]{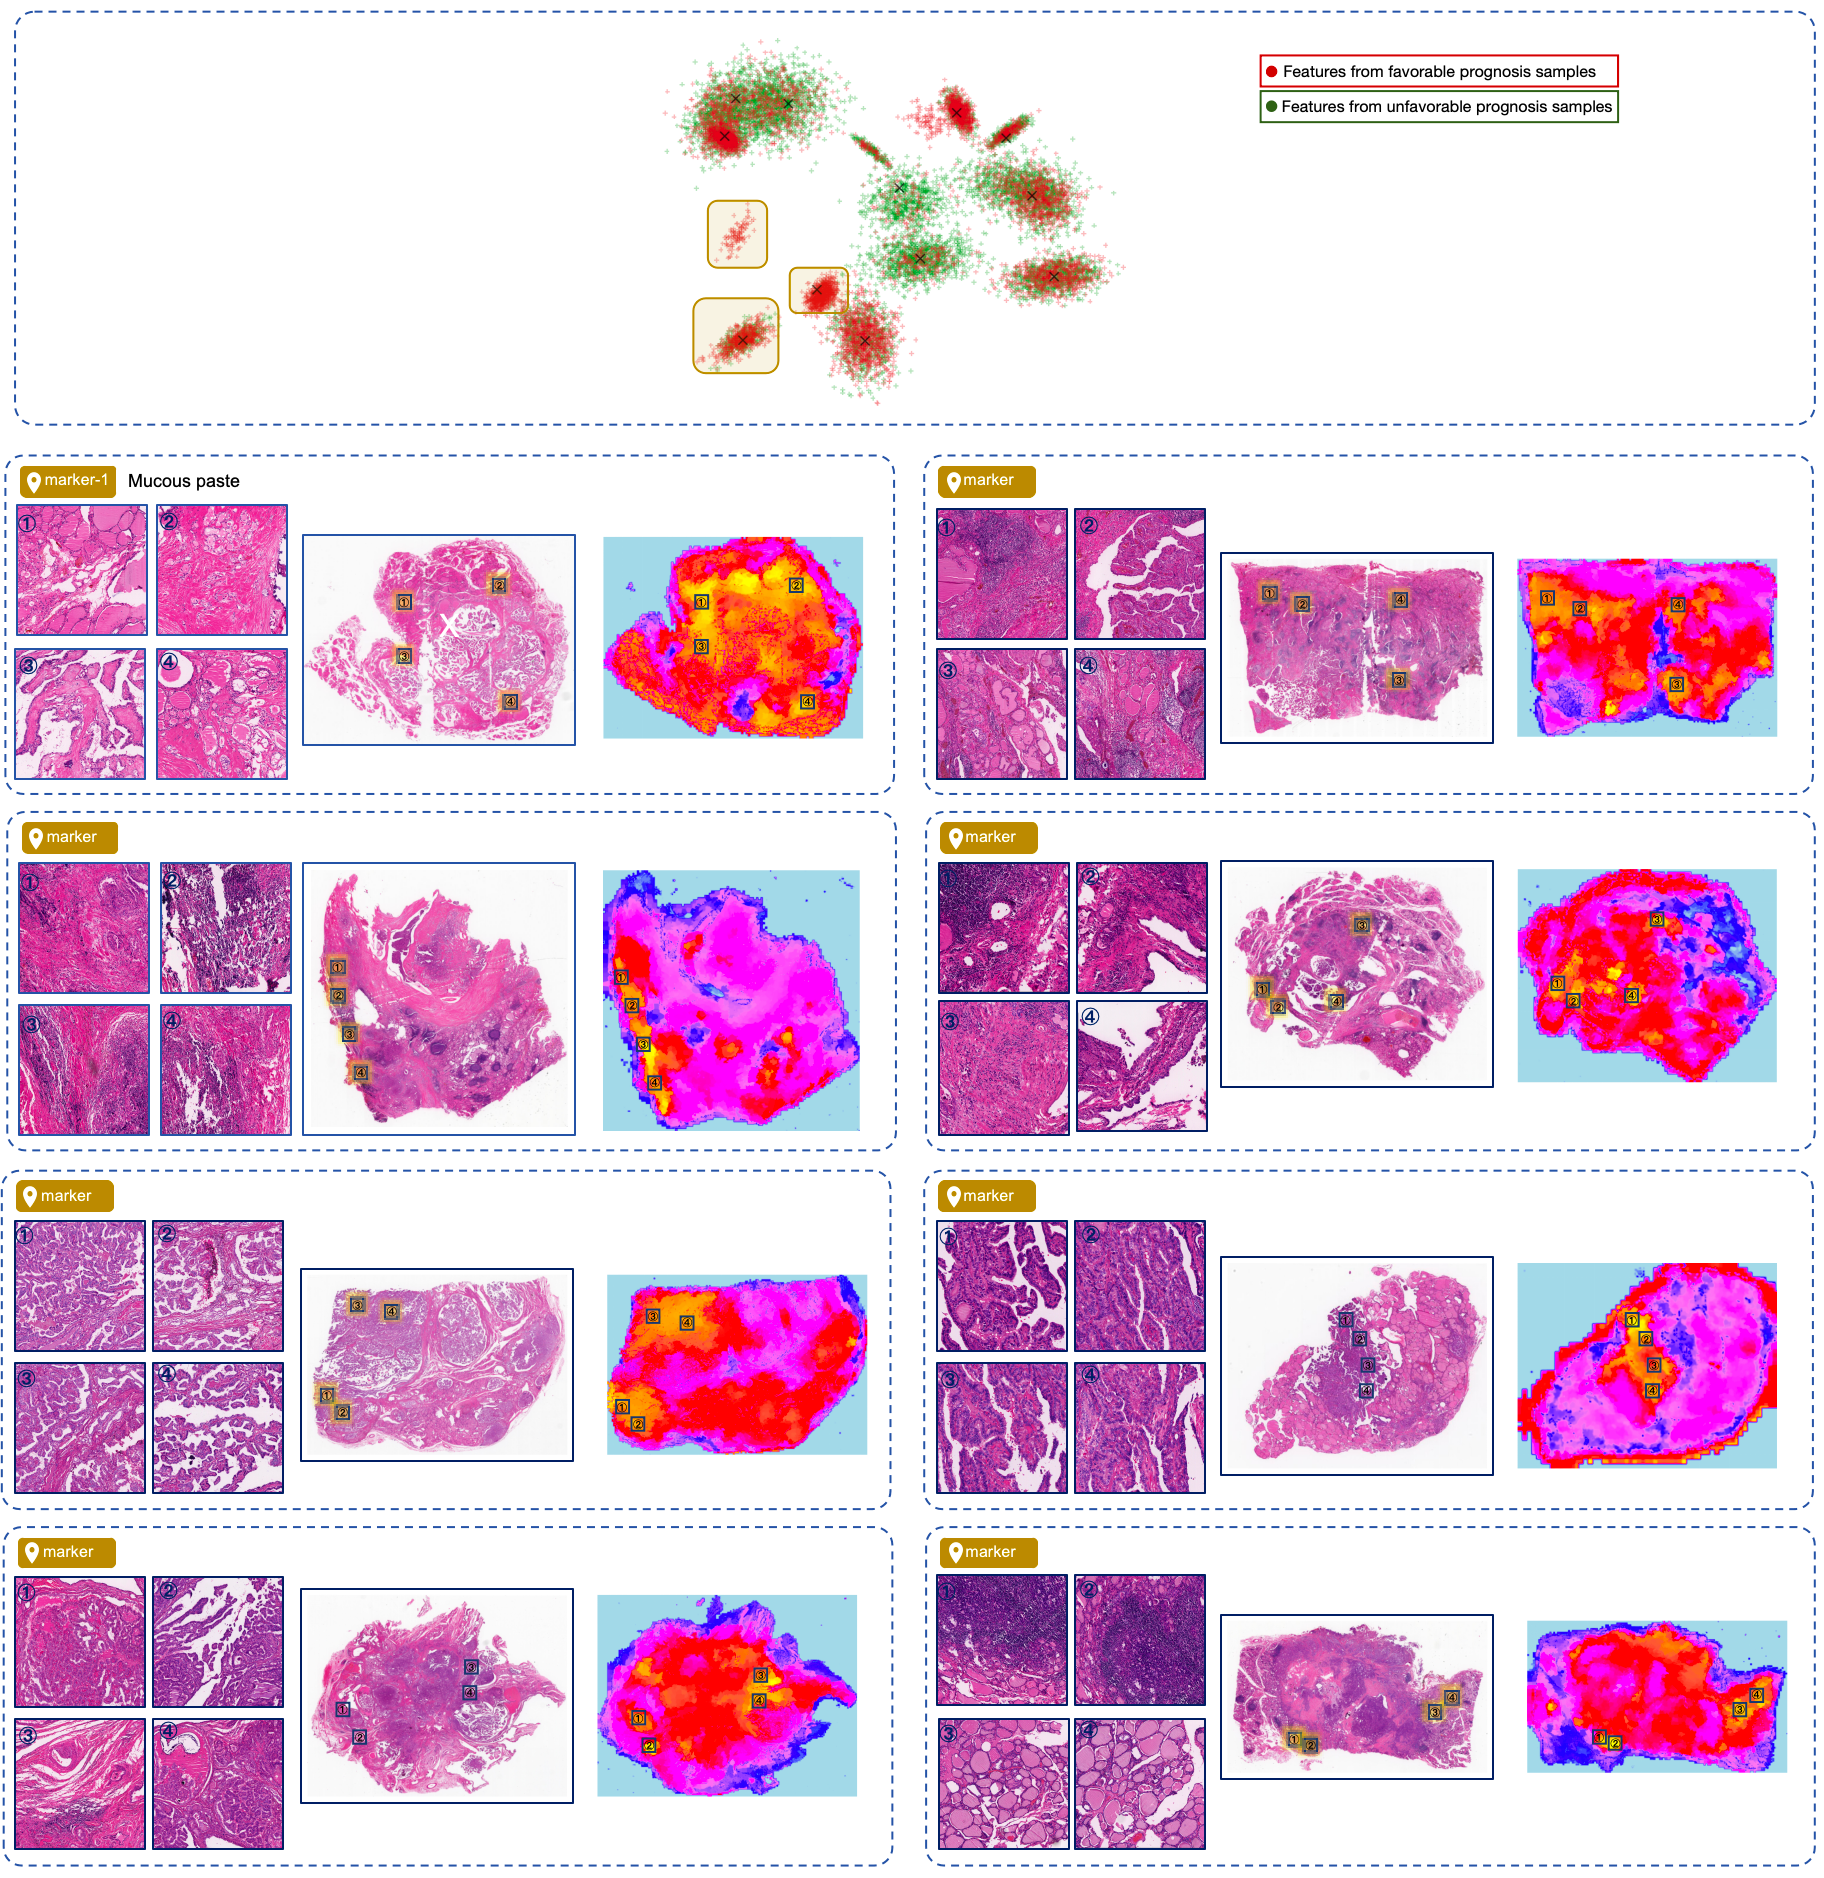}
    \caption{
    Visualization of mined tumor markers in thyroid cancer samples:  The SEW model is employed to extract pathological tissue-scale features from focused areas of colorectal cancer samples and perform clustering analysis, with particular emphasis on two feature clusters (with only red points) linked to poor prognosis. then show some novel tumor markers (verified by the pathologist) identified in the WSIs, along with their corresponding locations. 
    } 
    \label{fig:visual3}
\end{figure*}
\begin{figure*}[!h]
    \includegraphics[width=0.92\textwidth]{fig/visualization_sup.pdf}
     \caption{In the SEW, the focusing module generates a visualization of the heatmap, as well as a detailed display of the high-risk area after magnification. For each magnified area, SEW performs clustering on the corresponding sub-graph node embeddings of this area to obtain a series of pathological prototypes. Clustering information is used to reconstruct high-risk areas, with different colors representing tissue areas of possibly different natures. Figures (a)、(b) and (c) are positive slides (lesion areas are outlined in red), while (d) are negative slides.} 
    \label{fig:visual}
\end{figure*}

\section*{C. Visualization Results}
\label{Visualization}
This section demonstrates the visualization results of SEW on HCC. The visualization was conducted on six positive and negative samples. In HCC, each slide is constructed into a super-pixel graph. Subsequently, the focus module assesses the pathological risk of each node, and a focus heatmap is drawn based on the scores obtained. Several high-risk areas are magnified, and within the magnified area, results are generated based on the acquired features using clustering techniques to identify pathological prototypes.the heatmap and clustering reconstruction results are displayed in Figure~\ref{fig:visual}.

This section showcases the visualization results of SEW on HCC. The visualization was conducted on six positive and negative samples. In HCC, each slide is constructed into a super-pixel graph. Subsequently, the focus module scores the importance of each node for the diagnostic outcome, with focus scores displayed on a heatmap with a gradient from yellow to blue. Several high-risk areas are magnified, and within the magnified area, results are generated based on the acquired features using clustering techniques to identify pathological prototypes. Then, the high-risk areas are reconstructed according to these clustering results, and the heatmap and clustering reconstruction results are displayed in Figure~\ref{fig:visual}.

From the visualization results, it is observed that SEW can focus on nodes with pathological changes (or those most suspicious for pathological changes) in both positive and negative samples. Through focusing, the magnified areas are trained on regions with sufficient tissue or cellular-level information. Additionally, the visualization results show that most areas are unimportant or repetitive. By focusing on only a few areas, SEW can save time during the training and inference stages.

In positive samples, the focus module assigns high scores to almost all pathological areas, with the super-pixel area receiving the highest score being magnified for accurate classification via the super-pixel graph classification method. SEW identifies several high-scoring areas to achieve precise whole-slide categorization, thereby enhancing procedural efficiency and conserving storage space by ignoring low-scoring areas.

For each slide featuring a high-risk subgraph, pathological prototypes are identified using clustering techniques. Subsequently, high-risk areas are reconstructed based on these clustering results, employing different colors to represent tissue regions with distinct characteristics. This approach facilitates effective visualization of tissue composition within the magnified area for clinical diagnostics
\clearpage
{
    \small
    \bibliographystyle{ieeenat_fullname}
    \bibliography{main}
}
